# Supplementary material for: How to Solve Contextual Goal-Oriented Problems with Offline Datasets?
Source: arXiv:2408.07753 source file (2025-04-30)
Supplement: Supplementary file 1 [file appendix.tex]

\section{Proofs}
\label{app:proofs}
% \subsection{Proof of Lemma~\ref{lemma: upper_bound}}

\subsection{Proof of Lemma~\ref{lemma: decompose}}
\label{app:decomposition}
Our goal is to show that for any trajectory $\{c,s_h, a_h\}, h\in [T]$, we have
\begin{equation}
\begin{aligned}
&\sum_{h=1}^T(\phi(c,s_h,a_h)^\top\Lambda^{-1}\phi(c,s_h,a_h))^{1/2} \\
&\leq \sum_{h=1}^{T}[\mathbf{1}(a_h \neq a^+)(\phi_P(s_h,a_h)^\top\Lambda_P^{-1}\phi_P(s_h,a_h))^{1/2} + \mathbf{1}(a_h = a^+)(\bar{\phi}_R(c,s_h)^\top\Lambda^{-1}_R\bar{\phi}_R(c,s_h))^{1/2}].
\end{aligned}
\end{equation}
Recall that 
\begin{equation}
\begin{aligned}
&\Lambda=\sum_{i=1}^{N+N'}(\phi(c_i,s_i,a_i)\phi(c_i,s_i,a_i)^\top + \lambda I)\\
&= \sum_{i=1}^N\begin{bmatrix}
    \phi_{P}(s_i,a_i)\\
    \mathbf{0}
\end{bmatrix}\begin{bmatrix}
    \phi_{P}(s_i,a_i)\\
    \mathbf{0}
    \end{bmatrix}^\top + \sum_{i'=1}^{N'}\begin{bmatrix}
    \mathbf{0}\\
    \bar{\phi}_R(c_{i'},s_{i'})
\end{bmatrix}\begin{bmatrix}
    \mathbf{0}\\
    \bar{\phi}_R(c_{i'},s_{i'})
\end{bmatrix}^\top + \lambda I.
\end{aligned}
\end{equation}

\paragraph{1.}We first consider the case when $a_h \neq a^+$. 

Let 
$A = \sum_{i=1}^N\begin{bmatrix}
    \phi_{P}(s_i,a_i)\\
    \mathbf{0}
\end{bmatrix}\begin{bmatrix}
    \phi_{P}(s_i,a_i)\\
    \mathbf{0}
    \end{bmatrix}^\top+\sum_{i'=1}^{N'-1}\begin{bmatrix}
    \mathbf{0}\\
    \bar{\phi}_R(c_{i'},s_{i'})
\end{bmatrix}\begin{bmatrix}
    \mathbf{0}\\
    \bar{\phi}_R(c_{i'},s_{i'})
\end{bmatrix}^\top+ \lambda I$.

From the Sherman–Morrison formula, we have 
\begin{equation}
\begin{aligned}
&\Lambda^{-1} = (A+\begin{bmatrix}
    \mathbf{0}\\
    \bar{\phi}_R(c_{N'},s_{N'})
\end{bmatrix}\begin{bmatrix}
    \mathbf{0}\\
    \bar{\phi}_R(c_{N'},s_{N'})
\end{bmatrix}^\top )^{-1}\\
& = A^{-1}- \frac{A^{-1}\begin{bmatrix}
    \mathbf{0}\\
    \bar{\phi}_R(c_{N'},s_{N'})
\end{bmatrix}\begin{bmatrix}
    \mathbf{0}\\
    \bar{\phi}_R(c_{N'},s_{N'})
\end{bmatrix}^\top A^{-1}}{1+\begin{bmatrix}
    \mathbf{0}\\
    \bar{\phi}_R(c_{N'},s_{N'})
\end{bmatrix}^\top A^{-1}
\begin{bmatrix}
    \mathbf{0}\\
    \bar{\phi}_R(c_{N'},s_{N'})
\end{bmatrix}
}
\end{aligned}
\end{equation}
where  $\frac{A^{-1}\begin{bmatrix}
    \mathbf{0}\\
    \bar{\phi}_R(c_{N'},s_{N'})
\end{bmatrix}\begin{bmatrix}
    \mathbf{0}\\
    \bar{\phi}_R(c_{N'},s_{N'})
\end{bmatrix}^\top A^{-1}}{1+\begin{bmatrix}
    \mathbf{0}\\
    \bar{\phi}_R(c_{N'},s_{N'})
\end{bmatrix}^\top A^{-1}
\begin{bmatrix}
    \mathbf{0}\\
    \bar{\phi}_R(c_{N'},s_{N'})
\end{bmatrix}
}$ is positive semi-definite. 

So we have:
\begin{equation}
\phi(c, s_h, a_h)^\top \Lambda^{-1}\phi(c, s_h, a_h) \leq \phi(c, s_h, a_h)^\top A^{-1}\phi(c, s_h, a_h).
\end{equation}
Repeating the above steps for $N'$ times we will have that for $a_h \neq a^+$
\begin{equation}
\begin{aligned}
&\phi(c, s_h, a_h)^\top \Lambda^{-1}\phi(c, s_h, a_h) \\
&\leq \phi(c, s_h, a_h)^\top \big(\sum_{i=1}^N\begin{bmatrix}
    \phi_{P}(s_i,a_i)\\
    \mathbf{0}
\end{bmatrix}\begin{bmatrix}
    \phi_{P}(s_i,a_i)\\
    \mathbf{0}
    \end{bmatrix}^\top + \lambda I\big)^{-1}\phi(c, s_h, a_h)\\
& = \begin{bmatrix}
    \phi_{P}(s_h,a_h)\\
    \mathbf{0}
\end{bmatrix}^\top \big(\sum_{i=1}^N\begin{bmatrix}
    \phi_{P}(s_i,a_i)\\
    \mathbf{0}
\end{bmatrix}\begin{bmatrix}
    \phi_{P}(s_i,a_i)\\
    \mathbf{0}
    \end{bmatrix}^\top + \lambda I\big)^{-1}\begin{bmatrix}
    \phi_{P}(s_h,a_h)\\
    \mathbf{0}
\end{bmatrix}.\\
\end{aligned}
\end{equation}
Let $B=\sum_{i=1}^N\begin{bmatrix}
    \phi_{P}(s_i,a_i)\\
    \mathbf{0}
\end{bmatrix}\begin{bmatrix}
    \phi_{P}(s_i,a_i)\\
    \mathbf{0}
    \end{bmatrix}^\top + \lambda I  = \begin{bmatrix}
    \sum_{i=1}^N\phi_{P}(s_i,a_i)\phi_{P}(s_i,a_i)^\top + \lambda I & \mathbf{0}\\
    \mathbf{0} & \lambda I
\end{bmatrix}$,

And $B^{-1} = \begin{bmatrix}
    (\sum_{i=1}^N\phi_{P}(s_i,a_i)\phi_{P}(s_i,a_i)^\top + \lambda I)^{-1} & \mathbf{0}\\
    \mathbf{0} & (\lambda I)^{-1}.
\end{bmatrix}$

As a result, when $a_h\neq a^+$,
\begin{equation}
\phi(c, s_h, a_h)^\top \Lambda^{-1}\phi(c, s_h, a_h)\leq \phi_P(s_h,a_h)^\top\Lambda_P^{-1}\phi_P(s_h,a_h),
\end{equation}
where
$\Lambda_P = \sum_{i=1}^N{\phi_P(s_i,a_i)\phi_P(s_i,a_i)^\top + \lambda I}$.

\paragraph{2.}When $a_h = a^+$, we can follow similar steps to show that 
\begin{equation}
\phi(c, s_h, a_h)^\top \Lambda^{-1}\phi(c, s_h, a_h)\leq     \bar{\phi}_R(c,s_h)^\top\Lambda^{-1}_R\bar{\phi}_R(c,s_h),
\end{equation}
where $\Lambda_R = \sum_{i'=1}^{N'}{\bar{\phi}_R(c_{i'},s_{i'})\bar{\phi}_R(c_{i'},s_{i'})^\top + \lambda I}$, which completes the proof.
\subsection{Proof of Theorem~\ref{theorem: coverage}}
\label{app:coverage}
Combining the result from Lemma~\ref{lemma: subopt} and Lemma~\ref{lemma: decompose}, w.p. at least $1-\xi$, for any $x\in \mathcal{S}$ and $c \in \mathcal{C}$, we have
\begin{equation}
\begin{aligned}
&\text{SubOpt}(\text{Pess}(D_\text{aug},x,c) \leq 2\beta \mathbb{E}_{\pi_c^*}\big[\sum_{h=1}^{T}[\mathbf{1}(a_h \neq a^+)(\phi_P(s_h,a_h)^\top\Lambda_P^{-1}\phi_P(s_h,a_h))^{1/2} \\
&+ \mathbf{1}(a_h = a^+)(\bar{\phi}_R(c,s_h)^\top\Lambda^{-1}_R\bar{\phi}_R(c,s_h))^{1/2}]|s_1 = x\big].    
\end{aligned}
\end{equation}

Since $\pi_c^*$ is the optimal policy, $a^+$ will only appear at the last step $h=T$ (which means it successfully reaches the goal) or never appears (no success). (If it applies $a^+$ before reaching the real goal set, there's always a better policy that does not perform $a^+$ to avoid the negative reward.)

If $a^+$ appears at $h=T$, we have
\begin{equation}
\begin{aligned}
&\sum_{h=1}^{T}[\mathbf{1}(a_h \neq a^+)(\phi_P(s_h,a_h)^\top\Lambda_P^{-1}\phi_P(s_h,a_h))^{1/2}+ \mathbf{1}(a_h = a^+)(\bar{\phi}_R(c,s_h)^\top\Lambda^{-1}_R\bar{\phi}_R(c,s_h))^{1/2}]\\
&= \sum_{h=1}^{T-1}(\phi_P(s_h,a_h)^\top\Lambda_P^{-1}\phi_P(s_h,a_h))^{1/2} + (\bar{\phi}_R(c,s_T)^\top\Lambda^{-1}_R\bar{\phi}_R(c,s_T))^{1/2}.
\end{aligned}
\end{equation}

If $a^+$ never appears in the trajectory, we have
\begin{equation}
\begin{aligned}
&\sum_{h=1}^{T}[\mathbf{1}(a_h \neq a^+)(\phi_P(s_h,a_h)^\top\Lambda_P^{-1}\phi_P(s_h,a_h))^{1/2}+ \mathbf{1}(a_h = a^+)(\bar{\phi}_R(c,s_h)^\top\Lambda^{-1}_R\bar{\phi}_R(c,s_h))^{1/2}]\\
&= \sum_{h=1}^{T}(\phi_P(s_h,a_h)^\top\Lambda_P^{-1}\phi_P(s_h,a_h))^{1/2}.
\end{aligned}
\end{equation}

Let $p(\text{success}|\pi_c^*)$ be the probability that  $\pi_c^*$ reaches the goal set given $c$ in the environment. Then we have
\begin{equation}
\begin{aligned}
&\mathbb{E}_{\pi_c^*}\big[\sum_{h=1}^{T}[\mathbf{1}(a_h \neq a^+)(\phi_P(s_h,a_h)^\top\Lambda_P^{-1}\phi_P(s_h,a_h))^{1/2}+ \mathbf{1}(a_h = a^+)(\bar{\phi}_R(c,s_h)^\top\Lambda^{-1}_R\bar{\phi}_R(c,s_h))^{1/2}]|s_1 = x\big]\\
&= p(\text{success}|\pi_c^*) \mathbb{E}_{\pi_c^*}\big[\sum_{h=1}^{T-1}(\phi_P(s_h,a_h)^\top\Lambda_P^{-1}\phi_P(s_h,a_h))^{1/2} + (\bar{\phi}_R(c,s_T)^\top\Lambda^{-1}_R\bar{\phi}_R(c,s_T))^{1/2} |s_1=x, \text{success}]\\
&+ (1-p(\text{success}|\pi_c^*))\mathbb{E}_{\pi_c^*}\big[\sum_{h=1}^{T}(\phi_P(s_h,a_h)^\top\Lambda_P^{-1}\phi_P(s_h,a_h))^{1/2}\big|s_1=x, \text{no success}].
\end{aligned}
\end{equation}
 
Recall event $\mathcal{E}^{\text{\textdagger}}$:
\begin{equation}
\begin{aligned}
&\mathcal{E}^{\text{\textdagger}}=\{\Lambda_P \geq I + c^{\text{\textdagger}}_0 N \mathbb{E}_{\pi^*_c}[\phi_P(s_h,a_h)\phi_P(s_h,a_h)^\top|s_1 = x, a_h \neq a^+, h\leq T] \\
&\text{and }\Lambda_R \geq I + c^{\text{\textdagger}}_1 N' \mathbb{E}_{\pi^*_c}[\bar{\phi}_R(c,s_h)\bar{\phi}_R(c, s_h)^\top|s_1 = x, a_h = a^+, h\leq T] \text{ for all $x\in\mathcal{S}$, $c \in \mathcal{C}$}\}. 
\end{aligned}
\end{equation}
Similar to the proof of Corollary 4.5 in~\cite{jin2021pessimism}, let $\Sigma_{h,P}(x) = \mathbb{E}_{\pi_c^*}[\phi_P(s_h,a_h)\phi_P(s_h,a_h)^\top|s_1=x, \text{success}]$, $\{\lambda_{h,j,P}(x)\}$ are the eigenvalues of $\Sigma_{h,P}(x)$.
From the assumption $\|\phi_P(s,a)\|\leq c_P$, we have 
\begin{equation}
    \|\Sigma_{h,P}(x)\|_{\text{op}} \leq \mathbb{E}_{\pi}[\|\phi_P(s_h,a_h)\phi_P(s_h,a_h)^\top\|_{\text{op}}|s_1=x, \text{success}] \leq c_P^2.
\end{equation}

On the event of $\varepsilon^{\text{\textdagger}}$, we have for any $h$,
\begin{equation}
\begin{aligned}
&\mathbb{E}_{\pi^*_c}[(\phi_P(s_h,a_h)^\top\Lambda_P^{-1}\phi_P(s_h,a_h))^{1/2}|s_1 =x, \text{success}]\\
&\leq \sqrt{\text{Tr}(\mathbb{E}_{\pi_c^*}[\phi_P(s_h,a_h)\phi_P(s_h,a_h)^\top |x_1=x, \text{success}]\Lambda_P^{-1})}\\
&\leq \sqrt{\Sigma_{h,P}(x)\big(I+c^{\text{\textdagger}}_0N\Sigma_{h,P}(x)\big)^{-1}}\\
&=\sqrt{\sum_{j=1}^{d_P}\frac{\lambda_{h, j, P}(x)}{1+c^{\text{\textdagger}}_0
N\lambda_{h, j, P}(x)}}\\
&\leq \sqrt{\sum_{j=1}^{d_P}\frac{c_P^2}{1+c^{\text{\textdagger}}_0c_P^2N}}
\end{aligned}
\end{equation}
where the first inequality comes from the Cauchy-Schwarz inequality, and the second inequality comes from the coverage assumption, the final inequality comes from the assumption that $\|\phi_P\|\leq c_P$.

Similarly, we have
\begin{equation}
\begin{aligned}
&\mathbb{E}_{\pi^*_c}[(\phi_P(s_h,a_h)^\top\Lambda_P^{-1}\phi_P(s_h,a_h))^{1/2}|s_1 =x, \text{no success}]\\
&\leq \sqrt{\sum_{j=1}^{d_P}\frac{c_P^2}{1+c^{\text{\textdagger}}_0c_P^2N}},
\end{aligned}
\end{equation}
for $h\in[T]$, and
\begin{equation}
\begin{aligned}
&\mathbb{E}_{\pi^*_c}[(\bar{\phi}_R(c,s_T)^\top\Lambda^{-1}_R\bar{\phi}_R(c,s_T))^{1/2}|s_1 =x, \text{success}]\\
&\leq \sqrt{\sum_{j=1}^{d_R+2}\frac{c_R^2}{1+c^{\text{\textdagger}}_1c_R^2N'}}.
\end{aligned}
\end{equation}

Combining the results above, we have
\begin{equation}
\begin{aligned}
&\mathbb{E}_{\pi_c^*}\big[\sum_{h=1}^{T}[\mathbf{1}(a_h \neq a^+)(\phi_P(s_h,a_h)^\top\Lambda_P^{-1}\phi_P(s_h,a_h))^{1/2}+ \mathbf{1}(a_h = a^+)(\bar{\phi}_R(c,s_h)^\top\Lambda^{-1}_R\bar{\phi}_R(c,s_h))^{1/2}]|s_1 = x\big]\\
&\leq p(\text{success}|\pi_c^*)\mathbb{E}_{\pi_c^*}[(T-1)\sqrt{\sum_{j=1}^{d_P}\frac{c_P^2}{1+c^{\text{\textdagger}}_0c_P^2N}} + \sqrt{\sum_{j=1}^{d_R+2}\frac{c_R^2}{1+c^{\text{\textdagger}}_1c_R^2N'}}]\\
&+(1-p(\text{success}|\pi_c^*))\mathbb{E}_{\pi_c^*}[T\sqrt{\sum_{j=1}^{d_P}\frac{c_P^2}{1+c^{\text{\textdagger}}_0c_P^2N}}]\\
&\leq p(\text{success}|\pi_c^*)\big(H_{\text{max}}\sqrt{\sum_{j=1}^{d_P}\frac{c_P^2}{1+c^{\text{\textdagger}}_0c_P^2N}} + \sqrt{\sum_{j=1}^{d_R+2}\frac{c_R^2}{1+c^{\text{\textdagger}}_1c_P^2N'}}\big)\\
&+(1-p(\text{success}|\pi_c^*))(H_{\text{max}}+1)\sqrt{\sum_{j=1}^{d_P}\frac{c_P^2}{1+c^{\text{\textdagger}}_0c_P^2N}}\\
&\leq (H_{\text{max}}+1)\sqrt{\sum_{j=1}^{d_P}\frac{c_P^2}{1+c^{\text{\textdagger}}_0c_P^2N}}+ \sqrt{\sum_{j=1}^{d_R+2}\frac{c_R^2}{1+c^{\text{\textdagger}}_1c_R^2N'}}.
\end{aligned}
\end{equation}

Define event $\mathcal{E}$:

\begin{equation}
\begin{aligned}
&\mathcal{E}=\{\text{SubOpt}(\text{Pess}(D_{\text{aug}}), x,c)\\
&\leq  \sum_{h=1}^{T}[\mathbf{1}(a_h \neq a^+)(\phi_P(s_h,a_h)^\top\Lambda_P^{-1}\phi_P(s_h,a_h))^{1/2} + \mathbf{1}(a_h = a^+)(\bar{\phi}_R(c,s_h)^\top\Lambda^{-1}_R\bar{\phi}_R(c,s_h))^{1/2}],
\end{aligned}
\end{equation}
which holds w.p. at least $1-\xi$.

Conditioned on $\mathcal{E}\cap \mathcal{E}^{\text{\textdagger}}$ and 
applying the definition of $\beta$, we have that 
\begin{equation}
\begin{aligned}
&\text{SubOpt}(\text{Pess}(D_{\text{aug}}), x,c)\\
&\leq 2\beta\big( (H_{\text{max}}+1)\sqrt{\sum_{j=1}^{d_P}\frac{c_P^2}{1+c^{\text{\textdagger}}_0c_P^2N}}+ \sqrt{\sum_{j=1}^{d_R+2}\frac{c_R^2}{1+c^{\text{\textdagger}}_1c_R^2N'}}\big)\\
&\leq c_1d^{3/2}\sqrt{\zeta}((H_{\text{max}}+1)^2N^{-1/2}+(H_{\text{max}}+1)N'^{-1/2}),
\end{aligned}
\end{equation}
where $c_1$ is some absolute constant only dependent on $c_P, c_R, c^{\text{\textdagger}}_0, c^{\text{\textdagger}}_1$ and $c_0$, $d = \max(d_{\phi_P}, d_{\phi_R}+2)$. The proof is then complete.

\subsection{Comparison with PDS~\citep{hu2023provable}}
\label{app:pds}
Suppose that we can learn a pessimistic linear reward function based on $\{c,s\}$ pairs to allow us to label reward for all $N$ real transitions given $c$. Following the CMDP construction, we can again construct a uniform representation $\phi_0(c,s,a)=\begin{bmatrix}
    \phi_P(s,a)\\
    \phi_R(c,s)
\end{bmatrix}$.

Let 
$\Lambda_0 = \sum_{j=1}^{N'} \sum_{i=1}^N{\phi_0(c_j, s_i,a_i)\phi_0(c_j, s_i,a_i)^\top + \lambda I}$, 

and 
$\Lambda_R = \sum_{j=1}^{N'}{\phi_R(c_j, s_j)\phi_R(c_j, s_j)^\top + \lambda I}$ (when learning the reward we can ignore the transition representation).

The coverage assumptions required by PDS are:
\begin{equation}
\{\Lambda_{R'} \geq I + c^{\text{\textdagger}}_2 N' \mathbb{E}_{\pi^*_c}[\phi_R(c,s_h)\phi_R(c, s_h)^\top|s_1 = x, h\leq T],\forall x\}
\end{equation} and 

\begin{equation}
\{\Lambda_0 \geq I + c^{\text{\textdagger}}_3 NN' \mathbb{E}_{\pi^*_c}[\phi_0(c,s_h,a_h)\phi_0(c, s_h,a_h)^\top|s_1 = x,h\leq T], \forall x \}
\end{equation}
where \textbf{the coverage assumption requires that the labeled dataset has sufficient coverage over the full trajectory generated by the optimal policy}. 

And under such coverage assumption, directly adapting Theorem 4.3 in~\cite{hu2023provable},  we have the upper bound:
\begin{equation}
\text{SubOpt}(\text{PDS}(\mathcal{D},\mathcal{D}'), x,c)\leq c_1H_{max}^2d_{\phi_0}^{3/2}\zeta_1^{1/2}(NN')^{-1/2} +c_2H_{max}d_{\phi_R}\zeta_2^{1/2}N'^{-1/2}.
\end{equation}
\ying{Here the $NN'$ term shows up since we cannot separate the reward and transition uncertainty. The extra $N'*$ should have no use in reducing the uncertainty in transition. So it could be hard to make the PDS case comparable to ours. The only thing we can say is the coverage assumption in eq. (30).}

\section{MBS-VI}

\label{app:mbs}

\subsection{Assumption 1} (Bounded densities). For any non-stationary policy $\pi$ and $h \geq 0$, $\eta_h^{\pi}(s; a) \leq U$.
Let $C=\frac{U}{b}$, $b$ is the hyperparameter.

\subsection{Assumption 2}
Density estimation error: see the decomposition below.
\paragraph{Mixture of densities} Let $\mu$ be a behavior distribution over ${\mathcal{S}} \times \mathcal{C} \times \bar{\mathcal{A}}$, $\mu_1$ over ${\mathcal{S}} \times \mathcal{C} \times \mathcal{A}$ (but $\mu_1$ is only dependent on ${\mathcal{S}}$, ${\mathcal{A}}$; for any $c\in\mathcal{C}$, $\mu_1$ is the same), and $\mu_2$ over $ {\mathcal{S}} \times \mathcal{C} \times \{a^+\} $. Notice that \textbf{two density functions has disjoint supports.}

Assume that our transitions dataset is from state-action distribution $\mu_1$ and our fake transition dataset is from state-action distribution $\mu_2$. Let $\mu(s,c,a) = w_1 \mu_1(s,c,a) + w_2 \mu_2(s,c,a)$ to be a mixture of the two distributions where $w_1 + w_2 = 1, w_1 >0, w_2>0$. ($\mu_1(s,c,a) = \mu_1(s,a)p(c)$).

% \textbf{Notice that $\mu_1$ and $\mu_2$ have disjoint supports}: actions are only in $\mathcal{A}$ for $\mu_1$, and in $\{a^+\}$ for $\mu_2$.

Let $\hat \mu = w_1 \hat \mu_1 + w_2 \hat \mu_2$
% Assume that we have $N$ i.i.d. samples from $\mu_1 \times R \times  P$, where $\mu_1$ is only nonzero when $a \neq a^+$; and we have $M$ i.i.d. sample from $\mu_2 \times \bar R \times \bar P$, where $\mu_2$ is only nonzero when $a = a^+$. Consider $\mu = \frac{N}{N+M} \mu_1 + \frac{M}{N+M} \mu_2$, we have $M+N$ samples from $\mu$.
, $\zeta (s,c,a,\hat{\mu}, b) = \mathbf{1} (\hat{\mu}(s,c,a)>b)$.

\paragraph{About $\epsilon_\mu$} Recall that $||\mu-\hat\mu||_{TV} \leq \epsilon_\mu$ w.p. $1-\delta$.

Density estimation error: w.p. $1-\delta$, $||\mu_1-\hat\mu_1||_{TV}\leq \epsilon_\mu^1$; w.p. $1-\delta$, $||\mu_2-\hat\mu_2||_{TV}\leq \epsilon_\mu^2$. Then w.p. at least $1-2\delta$,

\begin{equation}
\begin{split}
&\mathrel{\phantom{=}}||\mu-\hat\mu||_{TV} = \sup_{s,c,a} |\mu- \hat \mu| \\
&=\sup_{s,c,a}|w_1\mu_1 - w_1 \hat\mu_1 + w_2\mu_2 -w_2 \hat \mu_2|\\
&\leq \sup_{s,c,a}(|w_1\mu_1 - w_1 \hat\mu_1| + |w_2\mu_2 -w_2 \hat \mu_2|)\\
& \leq \sup_{s,c,a}|w_1\mu_1 - w_1 \hat\mu_1| +\sup_{s,c,a}|w_2\mu_2 -w_2 \hat \mu_2|\\
& = w_1 \epsilon_\mu^1+w_2\epsilon_\mu^2.
\end{split}
\end{equation}

\subsection{Assumption 3} 

\paragraph{About $\epsilon_\mathcal{F}$} 
Recall that $\epsilon_{\mathcal{F},\mu} = \max_{f\in\mathcal{F}}\min_{g\in\mathcal{F}}\mathbb{E}_{(s,c,a)\sim \mu}[||g(s,c,a) - \tilde{\Tau} f(s,c,a)||_2^2]$. 

Assume $\mathcal{F}_1$ to be function class from ${\mathcal{S}} \times \mathcal{C} \times \mathcal{A} \rightarrow \mathbb{R}$, and $\mathcal{F}_2$ to be function class from ${\mathcal{S}} \times \mathcal{C} \times \{a^+\} \rightarrow \mathbb{R}$. Let $\mathcal{F}$ to be the function class $\mathcal{F}_1 \times \mathcal{F}_2$, which contains all combinations of $\mathcal{F}_1 $ and $ \mathcal{F}_2$ (which allows us to take max and min under different supports separately). ($\mathcal{F}_2$ would be equivalent to a class of reward functions.)

% Define $\epsilon_{\mathcal{F}_1, \mu_1} =\max_{f\in \mathcal{F}_1} \min_{g\in\mathcal{F}_1}\mathbb{E}_{(s,c,a)\sim \mu_1}[||g(s,c,a) - \tilde{\Tau} f(s,c,a)||_2^2]$, 
% $\epsilon_{\mathcal{F}_2, \mu_2} =\max_{f\in \mathcal{F}_2} \min_{g\in\mathcal{F}_2}\mathbb{E}_{(s,c,a)\sim \mu_2}[||g(s,c,a) - \tilde{\Tau} f(s,c,a)||_2^2]$. 

Recall that $\tilde{\Tau} f(s,c,a) = r(s,c,a) + \gamma \mathbb{E}_{s'}[\max_{a'}\zeta \circ f(s',c,a')]$.

\begin{equation}
\begin{split}
&\mathrel{\phantom{=}}\max_{f\in\mathcal{F}}\min_{g\in\mathcal{F}}\int ||g(s,c,a) - \tilde{\Tau} f(s,c,a)||_2^2\mu(s,c,a)d(s,c,a)\\
&=\max_{f\in \mathcal{F}}\min_{g\in\mathcal{F}}\int ||g(s,c,a) - \tilde{\Tau} f(s,c,a)||_2^2 (w_1 \mu_1(s,c,a) + w_2 \mu_2(s,c,a)) d(s,c,a)\\
&= \max_{f\in \mathcal{F}}\left(\min_{g\in\mathcal{F}_1}\int_{ {\mathcal{S}} \times \mathcal{C} \times \mathcal{A}} ||g(s,c,a) - \tilde{\Tau} f(s,c,a)||_2^2 (w_1 \mu_1(s,c,a) ) d(s,c,a)) \right. \\
&\mathrel{\phantom{=}}+ \left. \min_{g\in\mathcal{F}_2}\int_{ {\mathcal{S}} \times \mathcal{C} \times \{a^+\}} ||g(s,c,a) - \tilde{\Tau} f(s,c,a)||_2^2  (w_2 \mu_2(s,c,a))d(s,c,a) \right)\\
& = \max_{f\in \mathcal{F}}\min_{g\in\mathcal{F}_1}\int_{{\mathcal{S}} \times \mathcal{C} \times \mathcal{A}} ||g(s,c,a) - \tilde{\Tau} f(s,c,a)||_2^2 (w_1 \mu_1(s,c,a) ) d(s,c,a))  \\
&\mathrel{\phantom{=}}+ \min_{g\in\mathcal{F}_2}\int_{ {\mathcal{S}} \times \mathcal{C} \times \{a^+\}} ||g(s,c,a) - r(s,c,a)||_2^2  (w_2 \mu_2(s,c,a))d(s,c,a) \\
% &=\max (\max_{f\in \mathcal{F}_1}\min_{g\in\mathcal{F}_1}\int_{{\mathcal{S}} \times \mathcal{C} \times \mathcal{A}} ||g(s,c,a) - \tilde{\Tau} f(s,c,a)||_2^2 (w_1 \mu_1(s,c,a) ) d(s,c,a)), \\
% &\mathrel{\phantom{=}}\mathrel{\phantom{=}}\mathrel{\phantom{=}}\mathrel{\phantom{=}}\max_{f\in \mathcal{F}_2}\min_{g\in\mathcal{F}_1}\int_{{\mathcal{S}} \times \mathcal{C} \times \mathcal{A}} ||g(s,c,a) - \tilde{\Tau} f(s,c,a)||_2^2 (w_1 \mu_1(s,c,a) ) d(s,c,a)))\\
% &\mathrel{\phantom{=}}+ \min_{g\in\mathcal{F}_2}\int_{ {\mathcal{S}} \times \mathcal{C} \times \{a^+\}} ||g(s,c,a) - r(s,c,a)||_2^2  (w_2 \mu_2(s,c,a))d(s,c,a) \\
&:=\epsilon_{\mathcal{F}}^1 + \epsilon_{\mathcal{F}}^2
\end{split}
\end{equation}
where the second last equation comes from $\tilde{\Tau} f(s,c,a) = r(s,c,a)$ for $a = a^+$.

The first line shows the completeness of $\mathcal{F}_1$ itself, the second line shows the completeness of $\mathcal{F}_1$ being able to model the reward class $\mathcal{F}_2$, and the last line is the completeness of $\mathcal{F}_2$ being able to model the real reward function.

% If $f$ is in $\mathcal{F}_2$, $\argmin_g$ should be in $\mathcal{F}_1$. If $f$ is in $\mathcal{F}_1$, $\argmin_g$ should also be in $\mathcal{F}_1$. So we have:
% \begin{equation}
% \begin{split}
% &\mathrel{\phantom{=}}\max_{f\in \mathcal{F}}\min_{g\in\mathcal{F}}\int ||g(s,c,a) - \tilde{\Tau} f(s,c,a)||_2^2\mu(s,c,a) d(s,c,a)\\  
% &=\mathrel{\phantom{=}}\max_{f\in \mathcal{F}}\min_{g\in\mathcal{F}_1}\int ||g(s,c,a) - \tilde{\Tau} f(s,c,a)||_2^2 \mu(s,c,a) d(s,c,a)\\
% &=
% \end{split}
% \end{equation}
% next?
\subsection{Optimal policy gap}

\paragraph{About $\epsilon_\zeta$} Recall $\zeta$-constrained policy set: Let $\Pi_C^{\text{all}}$ be the set of policies that satisfy $\text{Pr}(\zeta (s,c,a,\hat{\mu}, b)=0|\pi) \leq \epsilon_\zeta$, i.e., $\mathbb{E}_{s,c,a\sim \eta^\pi}[\mathbf{1}(\zeta (s,c,a,\hat{\mu}, b)=0)]$. ($c$ can be seen as given in initial state, and does not change through out the trajectory.)

We denote the density under $\pi$ under different supports: one that contains real actions in $\mathcal{A}$ as $\eta^\pi_1$, another that contains fake action $a^+$ as $\eta^\pi_2$.

\begin{equation}
\begin{split}
& \mathrel{\phantom{=}}\mathbb{E}_{s,c,a\sim \eta^\pi}[\mathbf{1}(\zeta (s,c,a,\hat{\mu}, b)=0)]\\
& = \int \mathbf{1}(\zeta (s,c,a,\hat{\mu}, b)=0) \eta^\pi(s,c,a) d(s,c,a)\\
&=\int_{ {\mathcal{S}} \times \mathcal{C} \times \mathcal{A}}\mathbf{1}(\zeta (s,c,a,\hat{\mu}, b)=0) \eta^\pi_1(s,c,a) d(s,c,a)+ \int_{ {\mathcal{S}} \times \mathcal{C} \times \{a^+\}}\mathbf{1}(\zeta (s,c,a,\hat{\mu}, b)=0) \eta^\pi_2(s,c,a) d(s,c,a),\\
\end{split}
\end{equation}
% expand \mu
which is decomposed to the sum of the probability under a policy of escaping to state-actions with insufﬁcient data under different supports.

\paragraph{About the optimal policy gap $\epsilon$} Recall we define $\epsilon$ as  $\text{Pr}(\mu(s,c,a)\leq 2b|\pi^*) \leq \epsilon$. 

We can decompose this gap in a similar way as we decompose $\epsilon_\zeta$. Denote the density under $\pi^*$ under different supports: one that contains real actions in $\mathcal{A}$ as $\eta^{\pi^*}_1$, another that contains fake action $a^+$ as $\eta^{\pi^*}_2$:

\begin{equation}
\begin{split}
& \text{Pr}(\mu(s,c,a)\leq 2b|\pi^*) = \mathbb{E}_{(s,c,a)\sim\eta_\pi^*}[\mathbf{1}(\zeta(s,c,a,\mu, b)=0)]\\
& = \int \mathbf{1}(\zeta (s,c,a,{\mu}, b)=0) \eta^{\pi^*}(s,c,a) d(s,c,a)\\
&=\int_{ {\mathcal{S}} \times \mathcal{C} \times \mathcal{A}}\mathbf{1}(\zeta (s,c,a,{\mu}, b)=0) \eta^{\pi^*}_1(s,c,a) d(s,c,a)+ \int_{ {\mathcal{S}} \times \mathcal{C} \times \{a^+\}}\mathbf{1}(\zeta (s,c,a,{\mu}, b)=0) \eta^{\pi^*}_2(s,c,a) d(s,c,a)\\
&:=\epsilon_1 + \epsilon_2
\end{split}
\end{equation}

\subsection{Final result}

\begin{equation}
\begin{aligned}
&\text{Pr}(\hat{\mu}(c,s,a)\leq b|\pi^*) \\
&\leq \epsilon_1 + \epsilon_2 + C(w_1 \epsilon_\mu^1+w_2\epsilon_\mu^2)\\
& := \epsilon_{\zeta}'
\end{aligned}
\end{equation}
Applying this to Theorem 2 in \cite{liu2020provably}, we have
\begin{equation}
v_{M}^{\bar{\pi_t}} \geq v_{M}^* -\Delta,
\end{equation}
where
% to be added. cleaning up the equation
% \begin{equation}
% \begin{split}
% \Delta = 
% \frac{2C(\mathcal{O}(\sqrt{\frac{}{}
% ))}{(1-\gamma)^2}
% \end{split}
% \end{equation}
% \section{Reward conversion}
% whether a state is terminal or not?
% terminal will be propagated using the value function
% for other states there's no propagation
% add cases when there's no intersection for exact match: add noises in robo states?
\section{Experimental details}
\subsection{Hyperparameters and settings}
\paragraph{IQL.}
\paragraph{PDS.}
\paragraph{UDS+reward learning.}

\section{More reward evaluations}
\section{OOD goal examples in the context-goal set}
